# Supplementary material for: Leveraging Model-based Trees as Interpretable Surrogate Models for Model Distillation
Source: arXiv:2310.03112 source file (2023-10-04)
Supplement: Supplementary file 2 [file appendix_old.tex]

\subsection{GUIDE replication}
To validate the R implementation of GUIDE, the selection bias simulation example from \citep{Loh.2002} was replicated for independent features. For this, GUIDE was simulated both without bootstrap bias correction and with correction in 1000 repetitions. All settings were chosen to the best of my knowledge as described in the paper. In Table \ref{tab:app_guide_selection_bias} the results from the paper are listed in the first two columns and in the following two columns the results from the replication. In the replication the features $x_1, x_2, x_2$ are also selected in the uncorrected version to a certain extent as splitting variables. However, the bias is notable. The effect of the bias correction can also be seen, although not as considerable as in the results from the paper. 

\begin{table}[!htb]
\centering
\begin{tabular}[t]{l|rr|rr}
\hline
  & original biased & original corrected & R biased & R corrected\\
\hline
$\textbf{x}_1$ & 0 & 178 & 106 & 143\\
$\textbf{x}_2$ & 0 & 232 & 129 & 180\\
$\textbf{x}_3$ & 0 & 200 & 118 & 179\\
$\textbf{x}_4$ & 469 & 181 & 293 & 224\\
$\textbf{x}_5$ & 531 & 209 & 354 & 274\\
\hline
\end{tabular}
\caption{Comparison of the results on selection bias and bias correction from the paper \citep{Loh.2002} with my R implementation}
\label{tab:app_guide_selection_bias}
\end{table}

\subsection{Selection bias correction approach SLIM} \label{app:selection_bias_correction}

By means of a simulation, I investigated how the number of quantiles (n.quantiles) used as potential splitpoints in SLIM affects the selection bias for numerical features. 
The data is defined as follows:
\begin{itemize}
    \item $\textbf{x}_1, \textbf{x}_2 \sim U(0,1)$
    \item $\textbf{x}_3$ uniformly distributed on equidistant grids of length 10, 25, 50 and 100 on the interval [0,1] (i.e. four different settings)
    \item $y \sim N(0,1)$
\end{itemize}

For each of the four simulation scenarios, SLIM trees are fitted  with  \\ n.quantiles $\in \{100, 75, 50, 25, 10, 2\}$ and one exact tree (each unique value as potential splitpoint) in each simulation run. The experiment is repeated 3000 times.

In Table \ref{tab:app_selection_bias_independence_grid} the frequency of the selected features and the resulting train and test mean MSE for the four different grid sizes and seven different values of n.quantiles is listed. There one can see that the selection bias in all the variations shown decreases with decreasing values of n.quantiles. However, if n.quantiles is chosen equal to the number of unique values of $\textbf{x}_3$ the selection bias does not seem to be completely eliminated. Only when n.quantiles is chosen smaller is selection bias no longer visible.

For the MSE, it can be observed that as the number of n.quantiles decreases, the $MSE_{train}$ increases and the $MSE_{test}$ decreases. 
That $MSE_{train}$ increases with decreasing n.quantiles was to be expected and is due to the fact that if fewer quantiles are used as potential splitpoint set, the optimal splitpoint may not fall into this set. 
The values of $MSE_{test}$ are not very meaningful here, as there is no dependency between the features and the target. This means that the forced split is merely an adjustment to the random error terms, which naturally look different on the test data. A better generalisation is therefore obtained in this case if the fit to the training errors is not exact. 

\begin{table}
\centering \footnotesize
\begin{tabular}[t]{|l|l|r|r|r|r|r|r|r|}
\hline
\theadfont\diagbox[width=7em, height=5em]{$\textbf{x}_3$ \\ gridsize}{n.quantiles}&
\thead{}&\thead{exact}&\thead{100}&\thead{75}&\thead{50}&\thead{25}&\thead{10}&\thead{2}\\
\hline
10 & $\textbf{x}_1$ & 1439 & 1388 & 1353 & 1309 & 1249 & 1120 & 1039\\
10 & $\textbf{x}_2$ & 1316 & 1222 & 1224 & 1217 & 1153 & 1033 & 969\\
10 & $\textbf{x}_3$ & 245 & 390 & 423 & 474 & 598 & 847 & 992\\
10 & $MSE_{train}$ & 0.9841 & 0.9850 & 0.9851 & 0.9855 & 0.9863 & 0.9877 & 0.9906\\
10 & $MSE_{test}$ & 1.0193 & 1.0180 & 1.01789 & 1.0174 & 1.0165 & 1.0154 & 1.0110\\
\hline
25 & $\textbf{x}_1$ & 1294 & 1206 & 1169 & 1133 & 1042 & 995 & 992\\
25 & $\textbf{x}_2$ & 1244 & 1154 & 1138 & 1088 & 1033 & 1006 & 1012\\
25 & $\textbf{x}_3$ & 462 & 640 & 693 & 779 & 925 & 999 & 996\\
25 & $MSE_{train}$ & 0.9827 & 0.9833 & 0.9835 & 0.9838 & 0.9844 & 0.9857 & 0.9897\\
25 & $MSE_{test}$ & 1.0208 & 1.0198 & 1.0197 & 1.0194 & 1.0187 & 1.0172 & 1.0129\\
\hline
50 & $\textbf{x}_1$ & 1246 & 1125 & 1085 & 1057 & 1043 & 1018 & 1043\\
50 & $\textbf{x}_2$ & 1120 & 1035 & 1018 & 984 & 955 & 948 & 950\\
50 & $\textbf{x}_3$ & 634 & 840 & 897 & 959 & 1002 & 1034 & 1007\\
50 & $MSE_{train}$ & 0.9833 & 0.9840 & 0.9841 & 0.9844 & 0.9849 & 0.9863 & 0.9902\\
50 & $MSE_{test}$ & 1.0189 & 1.0179 & 1.01770 & 1.0173 & 1.0164 & 1.0150 & 1.0108\\
\hline
100 & $\textbf{x}_1$ & 1105 & 989 & 998 & 981 & 967 & 942 & 977\\
100 & $\textbf{x}_2$ & 1138 & 1048 & 1010 & 1031 & 1048 & 1030 & 1026\\
100 & $\textbf{x}_3$ & 757 & 963 & 992 & 988 & 985 & 1028 & 997\\
100 & $MSE_{train}$ & 0.9826 & 0.9832 & 0.9834 & 0.9837 & 0.9844 & 0.9859 & 0.9898\\
100 & $MSE_{test}$ & 1.0166 & 1.0157 & 1.0155 & 1.0151 & 1.0146 & 1.0129 & 1.0087\\
\hline
\end{tabular}
\caption{Frequency of feature selection and mean MSE for four different grid sizes and seven different values of n.quantiles}
\label{tab:app_selection_bias_independence_grid}
\end{table}

The scenarios independence numeric and independence mixed from chapter \ref{selection} were also simulated with varying values of n.quantiles. The results are listed in Table \ref{tab:app_selection_bias_independence}. 
In the case of scenario independence numeric, the approach seems to be successful. However, here again, only with n.quantiles = 2 selection bias is no longer visible. In the independence mixed scenario, the frequencies also change, but with no value of n.quantiles  an approximately unbiased result is found. If n.quantiles is chosen too small, the bias turns in the other direction (i.e. categorical variables are preferably used for the first split). Within the numerical variables ($\textbf{x}_1 ,... \textbf{x}_3$) the balance seems to succeed. The binary variety $\textbf{x}_4$ is not chosen sufficiently often in any variant. For the MSE, the results correspond to those of the previous simulation.


\begin{table}[!htb]
\centering \footnotesize
\begin{tabular}[t]{|l|l|r|r|r|r|r|r|r|}
\hline
\theadfont\diagbox[width=7em, height=5em]{$\textbf{x}_3$ \\ scenario}{n.quantiles}&
\thead{}&\thead{exact}&\thead{100}&\thead{75}&\thead{50}&\thead{25}&\thead{10}&\thead{2}\\
\hline
numeric & x1 & 1062 & 957 & 946 & 913 & 875 & 808 & 757\\
numeric & x2 & 1033 & 919 & 899 & 879 & 828 & 759 & 757\\
numeric & x3 & 205 & 284 & 293 & 349 & 446 & 646 & 750\\
numeric & x4 & 700 & 840 & 862 & 859 & 851 & 787 & 736\\
numeric & $MSE_{train}$ & 0.9800 & 0.9807 & 0.9808 & 0.9812 & 0.9820 & 0.9836 & 0.9868\\
numeric & $MSE_{test}$ & 1.0194 & 1.0187 & 1.0182 & 1.0179 & 1.0170 & 1.0160 & 1.0112\\
\hline
mixed & x1 & 1259 & 1186 & 1185 & 1153 & 1095 & 954 & 458\\
mixed & x2 & 1248 & 1184 & 1150 & 1126 & 1034 & 891 & 485\\
mixed & x3 & 362 & 465 & 488 & 534 & 638 & 769 & 463\\
mixed & x4 & 19 & 25 & 28 & 29 & 35 & 55 & 203\\
mixed & x5 & 61 & 78 & 83 & 89 & 113 & 188 & 778\\
mixed & x6 & 50 & 61 & 65 & 68 & 84 & 142 & 612\\
mixed & $MSE_{train}$ & 0.9528 & 0.9535 & 0.9538 & 0.9541 & 0.9550 & 0.9567 & 0.9606\\
mixed & $MSE_{test}$ & 1.0515 & 1.0498 & 1.0493 & 1.0486 & 1.0475 & 1.0450 & 1.0399\\
\hline
\end{tabular}
\caption{Frequency of feature selection and mean MSE for scenarios selection bias independence numeric and independence mixed and seven different values of n.quantiles}
\label{tab:app_selection_bias_independence}
\end{table}


In order to investigate whether the correction approach, which seems to work at least for numerical variables, also leads to unbiased variable selection in the presence of interactions, the numerical vs numerical scenario from chapter \ref{selection_bias_interactions} is simulated for different values of n.quantiles. The results are listed in Table \ref{tab:app_selection_bias_interaction}. 

$x_3$ only takes on 11 different values in this scenario. In the independence case, it would therefore be expected that the selection bias decreases with a decreasing number of quantiles and is no longer recognisable at least for n.quantiles = 2. Here, however, a different picture emerges. If all possible splitpoints are included, the variable $\textbf{x}_1$ with more possible splitpoints is preferred, as expected. With decreasing values of n.quantiles the relationship changes, but no direct linear relationship can be seen. Rather, the selection bias reverses at n.quantiles $= 100$ and then increases sharply and decreases again somewhat at lower values. However, the bias seems to be smallest when all possible split points are used for the exhaustive search. 

From this we can conclude that unbiasedness in the independence case does not automatically lead to unbiasedness in the presence of interactions. 
However, it is precisely the selection bias in the case of present interactions that is important. Since the effect of the correction approach on the selection bias in the presence of interactions is hardly generally predictable, this approach is therefore not recommended. Instead, n.quantiles should be chosen with regard to the criteria train and test MSE and, if necessary, computational time.


\begin{table}[!htb]
\centering \footnotesize
\begin{tabular}[t]{l|r|r|r|r|r|r|r}
\hline
n.quantiles  & exact & 100 & 75 & 50 & 25 & 10 & 2\\
\hline
$\textbf{x}_1$ & 1643.0000 & 1272.0000 & 1135.0000 & 924.0000 & 447.0000 & 592.0000 & 1809.0000\\
\hline
$\textbf{x}_3$ & 1357.0000 & 1728.0000 & 1865.0000 & 2076.0000 & 2553.0000 & 2408.0000 & 1191.0000\\
\hline
$MSE_{train}$ & 0.0373 & 0.0375 & 0.0376 & 0.0377 & 0.0380 & 0.0379 & 0.0393\\
\hline
$MSE_{test}$ & 0.0391 & 0.0393 & 0.0393 & 0.0393 & 0.0392 & 0.0392 & 0.0404\\
\hline
\end{tabular}
\caption{Frequency of feature selection and mean MSE for scenario selection bias numerical vs numerical and seven different values of n.quantiles}
\label{tab:app_selection_bias_interaction}
\end{table}





\clearpage
\subsection{Simulation results}
\subsubsection{Basic scenarios}\label{app:basic_scenarios}

\paragraph{XGBoost configurations}
In Table \ref{tab:app_xgboost_config} the XGBoost hyperparameter settings, which were used for the simulation of the basic scenarios are listed.
\begin{table}[!htb]
    \centering
    \begin{tabular}{l|r|r|r}
    \hline
    & linear smooth & linear categorical & linear mixed \\
    \hline
    max\_depth & 5 & 3 & 5 \\
    eta & 0.5 & 0.5 & 0.5 \\
    alpha & 1 & 0.5 & 2 \\
    gamma & 2 & 1 & 3.5 \\
    nrounds & 400 & 350 & 500\\
    \hline
    \end{tabular}
    \caption{XGBoost hyperparameters for basic scenarios after hyperparametertuning}
    \label{tab:app_xgboost_config}
\end{table}


\paragraph{Simulation Results}
The Figures \ref{fig:app_tree_low_symmetry} and \ref{fig:app_tree_high_symmetry} each show an example of a SLIM tree with high and low symmetry on the scenario linear smooth with each 8 leafnodes. The value impr in the plot is the potential relative improvement of the objective through the best split for this node in relation to the improvement in the parent node. In the tree \ref{fig:app_tree_high_symmetry}, the required improvement of $10 \%$ in node 2 is just missed, which is why this node is not split further.
\begin{figure}[!htb]
    \centering    
    \includegraphics[width = 16cm]{Figures/simulations/chapter_5_simulation_study/basic_scenarios/linear_smooth/tree_high_symmetry.png}  
    \caption{SLIM tree with high symmetry on scenario linear smooth}
    \label{fig:app_tree_high_symmetry}
\end{figure}

\begin{figure}[!htb]
    \includegraphics[width = 16cm]{Figures/simulations/chapter_5_simulation_study/basic_scenarios/linear_smooth/tree_low_symmetry.png}
    \caption{SLIM tree with low symmetry on scenario linear smooth}
    \label{fig:app_tree_low_symmetry}
\end{figure}




\clearpage

In the following tables and figures the mean simulation results of the basic scenarios, which are not included in chapter \ref{simulation} are shown.
\begin{table}[!htb]
\centering \tiny
\begin{tabular}[t]{l|l|r|r|r|r|r|r|r|r|r}
\hline
black box & MBT & $impr$ & $alpha$ & n leaves & n leaves min & n leaves max &  $R^2_{train}$ & sd $R^2_{train}$ & $R^2_{test}$ & sd $R^2_{test}$\\
\hline
lm & SLIM & 0.15 & & 2.06 & 2 & 3 & 0.9650 & 0.0043 & 0.9631 & 0.0046\\
lm & SLIM & 0.10 & & 12.11 & 5 & 16 & 0.9965 & 0.0052 & 0.9958 & 0.0060\\
lm & SLIM & 0.05 & & 15.70 & 14 & 16 & 0.9995 & 0.0001 & 0.9993 & 0.0001\\
lm & GUIDE & 0.15 & & 2.07 & 2 & 3 & 0.9651 & 0.0044 & 0.9632 & 0.0049\\
lm & GUIDE & 0.10 & & 12.03 & 5 & 16 & 0.9965 & 0.0051 & 0.9957 & 0.0060\\
lm & GUIDE & 0.05 & & 15.75 & 14 & 16 & 0.9995 & 0.0001 & 0.9993 & 0.0001\\
lm & MOB & & 0.001 & 15.78 & 14 & 16 & 0.9994 & 0.0001 & 0.9993 & 0.0001\\
lm & MOB & & 0.010 & 15.78 & 14 & 16 & 0.9994 & 0.0001 & 0.9993 & 0.0001\\
lm & MOB & & 0.050 & 15.78 & 14 & 16 & 0.9994 & 0.0001 & 0.9993 & 0.0001\\
lm & CTree & & 0.001 & 15.22 & 13 & 17 & 0.9993 & 0.0001 & 0.9992 & 0.0001\\
lm & CTree & & 0.010 & 15.22 & 13 & 17 & 0.9993 & 0.0001 & 0.9992 & 0.0001\\
lm & CTree & & 0.050 & 15.22 & 13 & 17 & 0.9993 & 0.0001 & 0.9992 & 0.0001\\
\hline
lm &  & & & & &  & 0.9902 & 0.0006 & 0.9901 & 0.0008\\
\hline

XGBoost & SLIM & 0.15 & & 2.31 & 2 & 6 & 0.9665 & 0.0069 & 0.9629 & 0.0079\\
XGBoost & SLIM & 0.10 & & 7.33 & 2 & 14 & 0.9850 & 0.0060 & 0.9814 & 0.0062\\
XGBoost & SLIM & 0.05 & & 14.30 & 8 & 17 & 0.9948 & 0.0010 & 0.9909 & 0.0017\\
XGBoost & GUIDE & 0.15 & & 2.26 & 2 & 5 & 0.9664 & 0.0067 & 0.9628 & 0.0077\\
XGBoost & GUIDE & 0.10 & & 6.92 & 2 & 14 & 0.9847 & 0.0061 & 0.9811 & 0.0062\\
XGBoost & GUIDE & 0.05 & & 14.15 & 8 & 17 & 0.9945 & 0.0010 & 0.9906 & 0.0017\\
XGBoost & MOB & & 0.001 & 10.89 & 8 & 13 & 0.9944 & 0.0005 & 0.9904 & 0.0011\\
XGBoost & MOB & & 0.010 & 11.96 & 9 & 15 & 0.9946 & 0.0005 & 0.9906 & 0.0011\\
XGBoost & MOB & & 0.050 & 12.86 & 11 & 15 & 0.9948 & 0.0005 & 0.9908 & 0.0011\\
XGBoost & CTree & & 0.001 & 12.09 & 9 & 15 & 0.9940 & 0.0006 & 0.9900 & 0.0012\\
XGBoost & CTree & & 0.010 & 13.21 & 10 & 15 & 0.9943 & 0.0006 & 0.9902 & 0.0013\\
XGBoost & CTree & & 0.050 & 14.09 & 11 & 17 & 0.9944 & 0.0006 & 0.9904 & 0.0012\\
\hline
XGBoost &  & & &  &  &  & 0.9858 & 0.0008 & 0.9768 & 0.0018\\
\hline
\end{tabular}
\caption{Mean simulation results on 100 simulation runs as surrogate models on scenario linear smooth with sample size $n = 1500$ for different values of $impr$ and $alpha$}
\label{tab:app_linear_smooth_1000}
\end{table}


\begin{figure}[!htb]
     \centering
    \includegraphics[width=14cm]{Figures/simulations/chapter_5_simulation_study/basic_scenarios/linear_smooth/ls_1000_standalone_symmetrie.png}
    \caption{Maximum leaf size of standalone MBTs vs number of leaf nodes scenario linear smooth with $n=1500, alpha = 0.001, impr = 0.1$}
\label{fig:app_ls_1000_standalone_symmetrie}
\end{figure} 


\begin{figure}[!htb]
     \centering
    \includegraphics[width=14cm]{Figures/simulations/chapter_5_simulation_study/basic_scenarios/linear_smooth/ls_1000_lm_r2_test.png}
    \caption{Test fidelity $R^2$ as surrogate on lm predictions vs number of leaf nodes scenario linear smooth with $n=1500, alpha = 0.001, impr = 0.1$}
\label{fig:app_ls_1000_lm_r2_test}
\end{figure} 

\begin{figure}[!htb]
     \centering     
    \includegraphics[width=14cm]{Figures/simulations/chapter_5_simulation_study/basic_scenarios/linear_smooth/ls_1000_xgboost_r2_test.png}
    \caption{Test fidelity $R^2$ as surrogate on XGBoost predictions vs number of leaf nodes scenario linear smooth with $n=1500, alpha = 0.001, impr = 0.1$}
    \label{fig:app_ls_1000_xgboost_r2_test}
\end{figure} 



\begin{table}[!htb]

\centering \tiny
\begin{tabular}[t]{l|l|r|r|r|r|r|r|r|r|r}
\hline
black box & MBT & $impr$ & $alpha$ & n leaves & n leaves min & n leaves max &  $R^2_{train}$ & sd $R^2_{train}$ & $R^2_{test}$ & sd $R^2_{test}$\\

\hline

standalone & SLIM & 0.15 & & 2.04 & 2 & 3 & 0.9542 & 0.0034 & 0.9536 & 0.0036\\
standalone & SLIM & 0.10 & & 36.94 & 15 & 58 & 0.9895 & 0.0024 & 0.9880 & 0.0024\\
standalone & SLIM & 0.05 & & 55.84 & 50 & 61 & 0.9910 & 0.0002 & 0.9890 & 0.0004\\
standalone & GUIDE & 0.15 & & 2.03 & 2 & 3 & 0.9540 & 0.0030 & 0.9534 & 0.0031\\
standalone & GUIDE & 0.10 & & 36.23 & 14 & 52 & 0.9894 & 0.0023 & 0.9881 & 0.0024\\
standalone & GUIDE & 0.05 & & 56.35 & 47 & 62 & 0.9909 & 0.0002 & 0.9891 & 0.0003\\
standalone & MOB & & 0.001 & 17.15 & 16 & 21 & 0.9901 & 0.0002 & 0.9893 & 0.0004\\
standalone & MOB & & 0.010 & 19.14 & 16 & 22 & 0.9902 & 0.0002 & 0.9894 & 0.0004\\
standalone & MOB & & 0.050 & 21.71 & 18 & 26 & 0.9903 & 0.0002 & 0.9895 & 0.0004\\
standalone & CTree & & 0.001 & 19.19 & 17 & 22 & 0.9901 & 0.0002 & 0.9894 & 0.0004\\
standalone & CTree &0 & 0.010 & 21.58 & 17 & 25 & 0.9902 & 0.0002 & 0.9895 & 0.0004\\
standalone & CTree & & 0.050 & 24.56 & 21 & 30 & 0.9903 & 0.0002 & 0.9895 & 0.0003\\


\hline
lm & SLIM & 0.15 & & 2.00 & 2 & 2 & 0.9628 & 0.0009 & 0.9625 & 0.0012\\
lm & SLIM & 0.10 & & 52.19 & 43 & 60 & 0.9999 & 0.0001 & 0.9998 & 0.0001\\
lm & SLIM & 0.05 & & 63.99 & 63 & 64 & 1.0000 & 0.0000 & 1.0000 & 0.0000\\
lm & GUIDE & 0.15 &  & 2.00 & 2 & 2 & 0.9628 & 0.0009 & 0.9625 & 0.0012\\
lm & GUIDE & 0.10 &  & 52.37 & 43 & 60 & 0.9999 & 0.0001 & 0.9998 & 0.0001\\
lm & GUIDE & 0.05 & & 63.99 & 63 & 64 & 1.0000 & 0.0000 & 1.0000 & 0.0000\\
lm & MOB & & 0.001 & 64.00 & 64 & 64 & 1.0000 & 0.0000 & 1.0000 & 0.0000\\
lm & MOB & & 0.010 & 64.00 & 64 & 64 & 1.0000 & 0.0000 & 1.0000 & 0.0000\\
lm & MOB & & 0.050 & 64.00 & 64 & 64 & 1.0000 & 0.0000 & 1.0000 & 0.0000\\
lm & CTree & & 0.001 & 63.60 & 62 & 64 & 1.0000 & 0.0000 & 1.0000 & 0.0000\\
lm & CTree & & 0.010 & 63.60 & 62 & 64 & 1.0000 & 0.0000 & 1.0000 & 0.0000\\
lm & CTree &5 & 0.050 & 63.60 & 62 & 64 & 1.0000 & 0.0000 & 1.0000 & 0.0000\\
\hline
lm & & & & & & & 0.9901 & 0.0002 & 0.9901 & 0.0003\\
\hline



XGBoost & SLIM & 0.15 & & 2.22 & 2 & 7 & 0.9647 & 0.0063 & 0.9643 & 0.0063\\
XGBoost & SLIM & 0.10 & & 19.23 & 3 & 40 & 0.9908 & 0.0062 & 0.9902 & 0.0062\\
XGBoost & SLIM & 0.05 & & 49.05 & 34 & 56 & 0.9978 & 0.0003 & 0.9972 & 0.0003\\
XGBoost & CTree & 0.15 & & 32.81 & 26 & 41 & 0.9972 & 0.0002 & 0.9965 & 0.0003\\
XGBoost & CTree & 0.10 & & 36.36 & 29 & 43 & 0.9973 & 0.0002 & 0.9966 & 0.0003\\
XGBoost & CTree & 0.05 & & 39.37 & 32 & 47 & 0.9974 & 0.0002 & 0.9967 & 0.0003\\
XGBoost & MOB & & 0.001 & 38.44 & 29 & 47 & 0.9979 & 0.0002 & 0.9972 & 0.0003\\
XGBoost & MOB & & 0.010 & 42.62 & 31 & 53 & 0.9980 & 0.0002 & 0.9973 & 0.0003\\
XGBoost & MOB & & 0.050 & 46.02 & 39 & 55 & 0.9981 & 0.0002 & 0.9974 & 0.0003\\
XGBoost & GUIDE & & 0.001 & 2.21 & 2 & 8 & 0.9645 & 0.0061 & 0.9641 & 0.0062\\
XGBoost & GUIDE & & 0.010 & 19.27 & 3 & 38 & 0.9907 & 0.0062 & 0.9900 & 0.0062\\
XGBoost & GUIDE & & 0.050 & 49.90 & 34 & 58 & 0.9977 & 0.0003 & 0.9970 & 0.0004\\
\hline
XGBoost & & & & & & & 0.9877 & 0.0003 & 0.9852 & 0.0006\\
\hline

\hline
\end{tabular}
\caption{Mean simulation results on 100 simulation runs as stand alone and surrogate models on scenario linear smooth with sample size $n = 7500$ for different values of $impr$ and $alpha$}
\label{tab:app_linear_smooth_5000}

\end{table}



\begin{table}[!htb]

\centering \tiny
\begin{tabular}[t]{l|l|r|r|r|r|r|r|r|r|r}
\hline
black box & MBT & $impr$ & $alpha$ & n leaves & n leaves min & n leaves max &  $R^2_{train}$ & sd $R^2_{train}$ & $R^2_{test}$ & sd $R^2_{test}$\\
\hline
gam & SLIM & 0.15 & & 2.00 & 2 & 2 & 0.8528 & 0.0064 & 0.8513 & 0.0108\\
gam & SLIM & 0.10 & & 2.64 & 2 & 4 & 0.8972 & 0.0432 & 0.8937 & 0.0440\\
gam & SLIM & 0.05 & & 8.56 & 4 & 16 & 0.9910 & 0.0029 & 0.9893 & 0.0039\\
gam & GUIDE & 0.15 & & 2.00 & 2 & 2 & 0.8528 & 0.0064 & 0.8513 & 0.0108\\
gam & GUIDE & 0.10 & & 2.64 & 2 & 4 & 0.8972 & 0.0432 & 0.8937 & 0.0440\\
gam & GUIDE & 0.05 & & 6.06 & 4 & 13 & 0.9875 & 0.0031 & 0.9859 & 0.0038\\
gam & MOB & & 0.001 & 13.53 & 11 & 15 & 0.9773 & 0.0020 & 0.9718 & 0.0028\\
gam & MOB & & 0.010 & 14.28 & 13 & 16 & 0.9784 & 0.0020 & 0.9728 & 0.0029\\
gam & MOB & & 0.050 & 14.92 & 13 & 16 & 0.9797 & 0.0021 & 0.9740 & 0.0028\\
gam & CTree & & 0.001 & 13.89 & 11 & 16 & 0.9773 & 0.0018 & 0.9720 & 0.0028\\
gam & CTree & & 0.010 & 14.47 & 12 & 16 & 0.9779 & 0.0017 & 0.9725 & 0.0027\\
gam & CTree & & 0.050 & 14.86 & 13 & 16 & 0.9783 & 0.0016 & 0.9729 & 0.0028\\
\hline
gam & & & & & & & 0.9702 & 0.0018 & 0.9694 & 0.0029\\
\hline

XGBoost & SLIM & 0.15 & & 2.00 & 2 & 2 & 0.8321 & 0.0075 & 0.8323 & 0.0118\\
XGBoost & SLIM & 0.10 & & 4.00 & 4 & 4 & 0.9923 & 0.0012 & 0.9870 & 0.0029\\
XGBoost & SLIM & 0.05 & & 4.00 & 4 & 4 & 0.9923 & 0.0012 & 0.9870 & 0.0029\\
XGBoost & GUIDE & 0.15 & & 2.00 & 2 & 2 & 0.8321 & 0.0075 & 0.8323 & 0.0118\\
XGBoost & GUIDE & 0.10 & & 4.00 & 4 & 4 & 0.9923 & 0.0012 & 0.9870 & 0.0029\\
XGBoost & GUIDE & 0.05 & & 4.00 & 4 & 4 & 0.9923 & 0.0012 & 0.9870 & 0.0029\\
XGBoost & MOB & & 0.001 & 13.45 & 11 & 16 & 0.9793 & 0.0063 & 0.9729 & 0.0069\\
XGBoost & MOB & & 0.010 & 14.38 & 13 & 16 & 0.9831 & 0.0055 & 0.9765 & 0.0066\\
XGBoost & MOB & & 0.050 & 14.63 & 13 & 16 & 0.9837 & 0.0052 & 0.9771 & 0.0062\\
XGBoost & CTree & & 0.001 & 11.96 & 10 & 14 & 0.9602 & 0.0030 & 0.9545 & 0.0049\\
XGBoost & CTree & & 0.010 & 12.76 & 10 & 15 & 0.9612 & 0.0033 & 0.9550 & 0.0050\\
XGBoost & CTree & & 0.050 & 13.46 & 10 & 16 & 0.9623 & 0.0036 & 0.9558 & 0.0052\\
\hline
XGBoost & & & & & & & 0.9876 & 0.0015 & 0.9778 & 0.0031\\
\hline
\end{tabular}
\caption{Mean simulation results on 100 simulation runs as surrogate models  on scenario linear categorical with sample size $n=1500$ for different values of $impr$ and $alpha$}
\label{tab:app_linear_abrupt_1000}

\end{table}



\begin{table}[!htb]

\centering \tiny
\begin{tabular}[t]{l|l|r|r|r|r|r|r|r|r|r}
\hline
black box & MBT & $impr$ & $alpha$ & n leaves & n leaves min & n leaves max &  $R^2_{train}$ & sd $R^2_{train}$ & $R^2_{test}$ & sd $R^2_{test}$\\
\hline
standalone & SLIM & 0.15 & & 2.00 & 2 & 2 & 0.8277 & 0.0032 & 0.8267 & 0.0048\\
standalone & SLIM & 0.10 & & 4.00 & 4 & 4 & 0.9887 & 0.0008 & 0.9886 & 0.0011\\
standalone & SLIM & 0.05 & & 4.00 & 4 & 4 & 0.9887 & 0.0008 & 0.9886 & 0.0011\\
standalone & GUIDE & 0.15 & & 2.00 & 2 & 2 & 0.8277 & 0.0032 & 0.8267 & 0.0048\\
standalone & GUIDE & 0.10 & & 4.00 & 4 & 4 & 0.9887 & 0.0008 & 0.9886 & 0.0011\\
standalone & GUIDE & 0.05 & & 4.00 & 4 & 4 & 0.9887 & 0.0008 & 0.9886 & 0.0011\\
standalone & MOB & & 0.001 & 41.23 & 26 & 48 & 0.9896 & 0.0004 & 0.9868 & 0.0011\\
standalone & MOB & & 0.010 & 45.50 & 27 & 53 & 0.9899 & 0.0003 & 0.9871 & 0.0011\\
standalone & MOB & & 0.050 & 49.24 & 31 & 58 & 0.9902 & 0.0003 & 0.9874 & 0.0011\\
standalone & CTree & & 0.001 & 22.51 & 20 & 25 & 0.9499 & 0.0014 & 0.9462 & 0.0022\\
standalone & CTree & & 0.010 & 24.39 & 21 & 27 & 0.9502 & 0.0014 & 0.9464 & 0.0023\\
standalone & CTree & & 0.050 & 26.62 & 22 & 30 & 0.9507 & 0.0016 & 0.9468 & 0.0023\\

\hline
gam & SLIM & 0.15 & & 2.00 & 2 & 2 & 0.8532 & 0.0029 & 0.8527 & 0.0043\\
gam & SLIM & 0.10 & & 2.22 & 2 & 4 & 0.8681 & 0.0299 & 0.8668 & 0.0302\\
gam & SLIM & 0.05 & & 27.66 & 13 & 42 & 0.9940 & 0.0036 & 0.9935 & 0.0039\\
gam & GUIDE & 0.15 & & 2.00 & 2 & 2 & 0.8532 & 0.0029 & 0.8527 & 0.0043\\
gam & GUIDE & 0.10 & & 2.22 & 2 & 4 & 0.8681 & 0.0299 & 0.8668 & 0.0302\\
gam & GUIDE & 0.05 & & 14.56 & 4 & 31 & 0.9886 & 0.0038 & 0.9882 & 0.0040\\
gam & MOB & & 0.001 & 61.11 & 55 & 64 & 0.9973 & 0.0002 & 0.9966 & 0.0003\\
gam & MOB & & 0.010 & 62.42 & 59 & 64 & 0.9973 & 0.0002 & 0.9966 & 0.0002\\
gam & MOB & & 0.050 & 63.15 & 61 & 64 & 0.9974 & 0.0002 & 0.9967 & 0.0002\\
gam & CTree & & 0.001 & 33.93 & 31 & 38 & 0.9789 & 0.0007 & 0.9769 & 0.0011\\
gam & CTree & & 0.010 & 36.76 & 34 & 43 & 0.9793 & 0.0008 & 0.9772 & 0.0012\\
gam & CTree & & 0.050 & 39.43 & 36 & 45 & 0.9798 & 0.0010 & 0.9776 & 0.0013\\

\hline
gam & & & & & & & 0.9701 & 0.0010 & 0.9698 & 0.0014\\
\hline

XGBoost & SLIM & 0.15 & & 2.00 & 2 & 2 & 0.8335 & 0.0033 & 0.8334 & 0.0048\\
XGBoost & SLIM & 0.10 & & 4.00 & 4 & 4 & 0.9949 & 0.0009 & 0.9942 & 0.0011\\
XGBoost & SLIM & 0.05 & & 4.00 & 4 & 4 & 0.9949 & 0.0009 & 0.9942 & 0.0011\\
XGBoost & GUIDE & 0.15 & & 2.00 & 2 & 2 & 0.8335 & 0.0033 & 0.8334 & 0.0048\\
XGBoost & GUIDE & 0.10 & & 4.00 & 4 & 4 & 0.9949 & 0.0009 & 0.9942 & 0.0011\\
XGBoost & GUIDE & 0.05 & & 4.00 & 4 & 4 & 0.9949 & 0.0009 & 0.9942 & 0.0011\\
XGBoost & MOB & & 0.001 & 53.91 & 49 & 60 & 0.9987 & 0.0002 & 0.9974 & 0.0007\\
XGBoost & MOB & & 0.010 & 55.38 & 49 & 60 & 0.9988 & 0.0002 & 0.9974 & 0.0007\\
XGBoost & MOB & & 0.050 & 56.40 & 50 & 61 & 0.9988 & 0.0002 & 0.9974 & 0.0007\\
XGBoost & CTree & & 0.001 & 24.16 & 19 & 29 & 0.9600 & 0.0016 & 0.9577 & 0.0021\\
XGBoost & CTree &  & 0.010 & 26.39 & 21 & 32 & 0.9605 & 0.0015 & 0.9581 & 0.0021\\
XGBoost & CTree & & 0.050 & 28.97 & 22 & 36 & 0.9612 & 0.0017 & 0.9587 & 0.0023\\
\hline
XGBoost & & & & & & & 0.9880 & 0.0009 & 0.9852 & 0.0009\\
\hline

\end{tabular}
\caption{Mean simulation results on 100 simulation runs as stand alone and surrogate models on scenario linear categorical with sample size $n = 7500$ for different values of $impr$ and $alpha$}
\label{tab:app_linear_abrupt_5000}

\end{table}




\begin{table}[!htb]

\centering \tiny
\begin{tabular}[t]{l|l|r|r|r|r|r|r|r|r|r}
\hline
black box & MBT & $impr$ & $alpha$ & n leaves & n leaves min & n leaves max &  $R^2_{train}$ & sd $R^2_{train}$ & $R^2_{test}$ & sd $R^2_{test}$\\
\hline
lm & SLIM & 0.15 & & 3.20 & 2 & 13 & 0.8879 & 0.0309 & 0.8806 & 0.0331\\
lm & SLIM & 0.10 & & 13.07 & 5 & 16 & 0.9875 & 0.0098 & 0.9843 & 0.0108\\
lm & SLIM & 0.05 & & 14.78 & 12 & 16 & 0.9913 & 0.0020 & 0.9885 & 0.0028\\
lm & GUIDE & 0.15 & & 3.17 & 2 & 13 & 0.8872 & 0.0308 & 0.8799 & 0.0329\\
lm & GUIDE & 0.10 & & 12.66 & 7 & 16 & 0.9866 & 0.0095 & 0.9834 & 0.0106\\
lm & GUIDE & 0.05 & & 14.38 & 12 & 16 & 0.9905 & 0.0022 & 0.9876 & 0.0029\\
lm & MOB & & 0.001 & 14.99 & 13 & 17 & 0.9882 & 0.0016 & 0.9838 & 0.0021\\
lm & MOB & & 0.010 & 14.99 & 13 & 17 & 0.9882 & 0.0016 & 0.9838 & 0.0021\\
lm & MOB & & 0.050 & 14.99 & 13 & 17 & 0.9882 & 0.0016 & 0.9838 & 0.0021\\
lm & CTree & & 0.001 & 15.05 & 13 & 17 & 0.9880 & 0.0016 & 0.9841 & 0.0019\\
lm & CTree & & 0.010 & 15.05 & 13 & 17 & 0.9880 & 0.0016 & 0.9841 & 0.0019\\
lm & CTree & & 0.050 & 15.05 & 13 & 17 & 0.9880 & 0.0016 & 0.9841 & 0.0019\\

\hline
lm & & & & & & & 0.9902 & 0.0006 & 0.9898 & 0.0008\\
\hline


XGBoost & SLIM & 0.15 & & 4.47 & 2 & 13 & 0.9067 & 0.0336 & 0.9013 & 0.0339\\
XGBoost & SLIM & 0.10 & & 12.80 & 7 & 16 & 0.9832 & 0.0089 & 0.9724 & 0.0103\\
XGBoost & SLIM & 0.05 & & 14.80 & 12 & 17 & 0.9870 & 0.0018 & 0.9764 & 0.0044\\
XGBoost & GUIDE & 0.15 & & 4.37 & 2 & 13 & 0.9059 & 0.0335 & 0.9005 & 0.0339\\
XGBoost & GUIDE & 0.10 & & 12.48 & 6 & 16 & 0.9822 & 0.0098 & 0.9715 & 0.0112\\
XGBoost & GUIDE & 0.05 & & 14.47 & 12 & 17 & 0.9863 & 0.0022 & 0.9758 & 0.0047\\
XGBoost & MOB & & 0.001 & 14.82 & 13 & 17 & 0.9853 & 0.0018 & 0.9745 & 0.0047\\
XGBoost & MOB & & 0.010 & 14.94 & 13 & 17 & 0.9854 & 0.0017 & 0.9746 & 0.0046\\
XGBoost & MOB & & 0.050 & 14.94 & 13 & 17 & 0.9854 & 0.0017 & 0.9746 & 0.0046\\
XGBoost & CTree & & 0.001 & 15.03 & 13 & 17 & 0.9850 & 0.0017 & 0.9743 & 0.0042\\
XGBoost & CTree & & 0.010 & 15.07 & 13 & 17 & 0.9850 & 0.0017 & 0.9743 & 0.0042\\
XGBoost & CTree & & 0.050 & 15.07 & 13 & 17 & 0.9850 & 0.0017 & 0.9743 & 0.0042\\
\hline
XGBoost & & & & & & & 0.9859 & 0.0014 & 0.9682 & 0.0042\\
\hline
\end{tabular}
\caption{Mean simulation results on 100 simulation runs as surrogate models on scenario linear mixed with sample size $n=1500$ for different values of $impr$ and $alpha$}
\label{tab:app_linear_mixed_1000}

\end{table}





\begin{table}[!htb]

\centering \tiny
\begin{tabular}[t]{l|l|r|r|r|r|r|r|r|r|r}
\hline
black box & MBT & $impr$ & $alpha$ & n leaves & n leaves min & n leaves max &  $R^2_{train}$ & sd $R^2_{train}$ & $R^2_{test}$ & sd $R^2_{test}$\\
\hline
standalone & SLIM & 0.15 & & 2.30 & 2 & 8 & 0.8637 & 0.0165 & 0.8626 & 0.0176\\
standalone & SLIM & 0.10 & & 38.96 & 21 & 54 & 0.9865 & 0.0029 & 0.9849 & 0.0030\\
standalone & SLIM & 0.05 & & 59.03 & 51 & 64 & 0.9904 & 0.0005 & 0.9884 & 0.0006\\
standalone & GUIDE & 0.15 & & 2.30 & 2 & 8 & 0.8637 & 0.0165 & 0.8626 & 0.0176\\
standalone & GUIDE & 0.10 & & 38.06 & 21 & 54 & 0.9866 & 0.0028 & 0.9851 & 0.0029\\
standalone & GUIDE & 0.05 & & 58.20 & 45 & 63 & 0.9903 & 0.0005 & 0.9885 & 0.0006\\
standalone & MOB & & 0.001 & 48.54 & 43 & 55 & 0.9888 & 0.0004 & 0.9861 & 0.0007\\
standalone & MOB & & 0.010 & 53.17 & 48 & 58 & 0.9891 & 0.0003 & 0.9864 & 0.0007\\
standalone & MOB & & 0.050 & 56.07 & 51 & 60 & 0.9893 & 0.0003 & 0.9866 & 0.0006\\
standalone & CTree & & 0.001 & 51.70 & 47 & 57 & 0.9887 & 0.0004 & 0.9858 & 0.0006\\
standalone & CTree & & 0.010 & 54.85 & 50 & 58 & 0.9889 & 0.0004 & 0.9860 & 0.0006\\
standalone & CTree & & 0.050 & 56.76 & 52 & 61 & 0.9890 & 0.0003 & 0.9860 & 0.0006\\

\hline
lm & SLIM & 0.15 & & 2.17 & 2 & 16 & 0.8683 & 0.0094 & 0.8677 & 0.0103\\
lm & SLIM & 0.10 & & 39.69 & 19 & 55 & 0.9956 & 0.0028 & 0.9953 & 0.0030\\
lm & SLIM & 0.05 & & 57.51 & 46 & 64 & 0.9991 & 0.0005 & 0.9990 & 0.0006\\
lm & GUIDE & 0.15 & & 2.17 & 2 & 16 & 0.8683 & 0.0094 & 0.8677 & 0.0103\\
lm & GUIDE & 0.10 & & 40.32 & 19 & 55 & 0.9960 & 0.0026 & 0.9956 & 0.0028\\
lm & GUIDE & 0.05 & & 57.32 & 46 & 64 & 0.9991 & 0.0005 & 0.9990 & 0.0006\\
lm & MOB & & 0.001 & 63.11 & 60 & 64 & 0.9973 & 0.0002 & 0.9964 & 0.0003\\
lm & MOB & & 0.010 & 63.11 & 60 & 64 & 0.9973 & 0.0002 & 0.9964 & 0.0003\\
lm & MOB & & 0.050 & 63.11 & 60 & 64 & 0.9973 & 0.0002 & 0.9964 & 0.0003\\
lm & CTree & & 0.001 & 62.72 & 59 & 64 & 0.9973 & 0.0002 & 0.9964 & 0.0003\\
lm & CTree & & 0.010 & 62.72 & 59 & 64 & 0.9973 & 0.0002 & 0.9964 & 0.0003\\
lm & CTree & & 0.050 & 62.72 & 59 & 64 & 0.9973 & 0.0002 & 0.9964 & 0.0003\\
\hline
lm & & & & & & & 0.9901 & 0.0003 & 0.9902 & 0.0004\\
\hline


\hline
XGBoost & SLIM & 0.15 & & 2.22 & 2 & 12 & 0.8693 & 0.0121 & 0.8706 & 0.0129\\
XGBoost & SLIM & 0.10 & & 39.52 & 23 & 53 & 0.9931 & 0.0027 & 0.9914 & 0.0027\\
XGBoost & SLIM & 0.05 & & 56.86 & 46 & 63 & 0.9964 & 0.0005 & 0.9948 & 0.0007\\
XGBoost & GUIDE & 0.15 & & 2.15 & 2 & 9 & 0.8693 & 0.0119 & 0.8705 & 0.0127\\
XGBoost & GUIDE & 0.10 & & 38.13 & 22 & 52 & 0.9928 & 0.0027 & 0.9912 & 0.0028\\
XGBoost & GUIDE & 0.05 & & 56.72 & 46 & 63 & 0.9963 & 0.0006 & 0.9946 & 0.0007\\
XGBoost & MOB & & 0.001 & 58.76 & 54 & 63 & 0.9961 & 0.0003 & 0.9942 & 0.0005\\
XGBoost & MOB & & 0.010 & 59.47 & 55 & 64 & 0.9961 & 0.0003 & 0.9943 & 0.0005\\
XGBoost & MOB & & 0.050 & 59.69 & 55 & 64 & 0.9961 & 0.0003 & 0.9943 & 0.0005\\
XGBoost & CTree & & 0.001 & 58.51 & 53 & 62 & 0.9956 & 0.0003 & 0.9936 & 0.0005\\
XGBoost & CTree & & 0.010 & 58.95 & 54 & 63 & 0.9956 & 0.0003 & 0.9936 & 0.0005\\
XGBoost & CTree & & 0.050 & 59.09 & 54 & 63 & 0.9956 & 0.0003 & 0.9936 & 0.0005\\
\hline
XGBoost & & & & & & & 0.9877 & 0.0007 & 0.9836 & 0.0011\\
\hline

\end{tabular}
\caption{Mean simulation results on 100 simulation runs as stand alone and surrogate models on scenario linear mixed with sample size $n = 7500$ for different values of $impr$ and $alpha$}
\label{tab:app_linear_mixed_5000}

\end{table}


\clearpage

\subsubsection{Linear smooth with noise features}
Figures \ref{fig:app_lasso_standalone_r2_test} and \ref{fig:app_lasso_standalone_r2_test_slim} show the the $R^2$ test accuracy in scenario linear smooth with noise features. Figure \ref{fig:app_lasso_standalone_r2_test_slim} shows that in this scenario asymmetric trees (i.e. trees with a maximum leafsize $> 700$) lead to poorer performance in SLIM and GUIDE.


\begin{figure}[!htb]
     \centering
     
    \includegraphics[width=16cm]{Figures/simulations/chapter_5_simulation_study/lasso/lasso_standalone_r2_test.png}
    \caption{Test accuracy $R^2$ of MBTs on scenario Linear smooth with noise features with $n=3000, alpha = 0.001, impr = 0.1$ with $n leaves \geq 11$}
    \label{fig:app_lasso_standalone_r2_test}
\end{figure} 

\begin{figure}[!htb]
     \centering
    \includegraphics[width=16cm]{Figures/simulations/chapter_5_simulation_study/lasso/lasso_standalone_r2_test_slim.png}
    \caption{Test accuracy $R^2$ of SLIM and GUIDE MBTs on scenario Linear smooth with noise features with $n=3000, alpha = 0.001, impr = 0.1$ with $n leaves \leq 11$}
\label{fig:app_lasso_standalone_r2_test_slim}
\end{figure} 

\subsubsection{Nonlinear effects}

\paragraph{XGBoost configurations}
In Table \ref{tab:app_xgboost_config_nonlinear} the XGBoost hyperparameter setting for simulation nonlinear is shown.
\begin{table}[!htb]
    \centering
    \begin{tabular}{l|r}
    \hline
    & nonlinear  \\
    \hline
    max\_depth & 4 \\
    eta & 0.825 \\
    alpha & 0.75 \\
    gamma & 1 \\
    nrounds & 700 \\
    \hline
    \end{tabular}
    \caption{XGBoost hyperparameters for scenario nonlinear after hyperparametertuning}
    \label{tab:app_xgboost_config_nonlinear}
\end{table}


\begin{table}[!htb]

\centering \tiny
\begin{tabular}[t]{l|l|r|r|r|r|r|r|r|r|r}
\hline
black box & model & n leaves & n l min & n l max & n split feat & n sf min & n sf max & \% main effect & df & sd df\\
\hline
standalone & basic lm & 43.06 & 36 & 48 & 5.68 & 4 & 6 & 0.5089 & 6.5804 & 0.1249\\
standalone & penalized poly & 19.32 & 16 & 22 & 4.26 & 3 & 5 & 0.2374 & 8.8768 & 0.3681\\
standalone & B-Splines & 18.38 & 13 & 22 & 4.26 & 3 & 6 & 0.0126 & & \\
standalone & gam & 17.60 & 12 & 22 & 3.44 & 2 & 4 & 0.0007 & & \\
\hline
XGBoost & basic lm & 30.38 & 2 & 47 & 4.56 & 1 & 6 & 0.6732 & 6.8519 & 0.1558\\
XGBoost & penalized poly & 20.66 & 16 & 24 & 4.70 & 3 & 6 & 0.2327 & 9.2909 & 0.4347\\
XGBoost & B-Splines & 17.38 & 2 & 25 & 4.70 & 1 & 6 & 0.0597 & &\\
XGBoost & gam & 15.28 & 2 & 24 & 4.00 & 1 & 6 & 0.0191 & &\\
\hline
\end{tabular}
\caption{Mean interpretability simulation results nonlinear variant 2}
\label{tab:app_nonlinear_interpretability}

\end{table}


\begin{table}[!htb] 

\centering \footnotesize
\begin{tabular}[t]{l|l|r|r|r|r|r}
\hline
black box & model & $R^2_{train}$  & sd $R^2_{train}$ & $R^2_{test}$ & sd $R^2_{test}$ & time in sec\\
\hline
standalone & basic lm & 0.9633 & 0.0035 & 0.9469 & 0.0048 & 102.2842\\
standalone & penalized poly & 0.9824 & 0.0015 & 0.9781 & 0.0020 & 195.4385\\
standalone & B-Splines & 0.9929 & 0.0013 & 0.9714 & 0.0029 & 113.2447\\
standalone & gam & 0.9880 & 0.0016 & 0.9835 & 0.0017 & 1544.3393\\
\hline
XGBoost & basic lm & 0.9198 & 0.0516 & 0.9030 & 0.0417 & 72.3790\\
XGBoost & penalized poly & 0.9750 & 0.0033 & 0.9634 & 0.0051 & 206.5870\\
XGBoost & B-Splines & 0.9865 & 0.0141 & 0.9591 & 0.0092 & 97.9321\\
XGBoost & gam & 0.9786 & 0.0127 & 0.9672 & 0.0115 & 1728.6021\\
\hline
XGBoost & XGBoost & 0.9392 & 0.0342 & 0.9216 & 0.0405 & 3.0131\\
\hline
\end{tabular}
\caption{Mean performance simulation results nonlinear effects variant 2}
\label{tab:app_nonlinear_performance}
\end{table}



\clearpage
\subsection{Insurance use case}
\subsubsection{K2204 BPV}

 \begin{figure}[!htb]
     \centering     
     \includegraphics[width = 14cm]{Figures/insurance_use_case/k2204_BPV/slim_lm_tree.png}
     \caption{SLIM tree with linear models as standalone model for BPV in data set K2204}
     \label{fig:app_ins_slim_lm_standalone_tree}
 \end{figure}

 \begin{figure}[!htb]
    \centering
    \includegraphics[width = 8cm]{Figures/insurance_use_case/k2204_BPV/hist_age.png}
    \caption{Frequency of observations with respect to feature age}
    \label{fig:app_ins_k2204_hist_age}
\end{figure}




\subsubsection{K2204 PPV}
All plots and tables shown in the chapter \ref{K2204_BPV} for the data set k2204 with target BPV are shown here for the target PPV (or PPV\_pred). The interpretation can be done analogously to chapter \ref{K2204_BPV}. The effects found here are merely all larger (since PPV is also larger than BPV) and their direction is exactly reversed. 

\begin{table}[!htb]
\centering \scriptsize
\begin{tabular}[t]{l|r|r|r|r|r}
\hline
  & $R^2$ & MSE & MAE & max AE & n leaves\\
\hline
linear baseline model & 0.985092 & 2.523500 & 1.277544 & 7.271319 & 1\\
\hline
SLIM & 0.999232 & 0.130069 & 0.255018 & 2.300768 & 8\\
GUIDE & 0.999275 & 0.122765 & 0.240393 & 2.300768 & 8\\
MOB & 0.998524 & 0.249776 & 0.353372 & 2.758192 & 8\\
CTree & 0.995088 & 0.831537 & 0.643819 & 4.808448 & 8\\
\hline
\end{tabular}
\label{tab:ins_k2204_ppv_lm_surrogates_perf}
\caption{Fidelity of K2204 PPV linear baseline model and linear MBTs}
\end{table}


\begin{table}[!htb]
\centering \scriptsize
\begin{tabular}[t]{l|r|r|r}
\hline
& age & duration & sex\\
\hline
SLIM & 0.28 & 0.67 & 0.05\\
GUIDE & 0.28 & 0.72 & 0.00\\
MOB & 0.10 & 0.77 & 0.13\\
CTree & 0.00 & 0.96 & 0.04\\
\hline
\end{tabular}
\label{tab:ins_k2204_ppv_lm_surrogates_share}
\caption{Share of observations split by the different features K2204 PPV linear MBTs}
\end{table}



Figure \ref{fig:ins_k2204_ppv_fit} plots the prediction of the baseline B-spline model and the two B-spline SLIM surrogates against PPV\_pred to visualise performance improvement. 

\begin{figure}[!htb]
    \centering    
    \includegraphics[width = 14cm]{Figures/insurance_use_case/k2204_PPV/fit.png}
    \caption{B-spline surrogate predictions vs. PPV\_pred for K2204}
    \label{fig:ins_k2204_ppv_fit}
\end{figure}

The fidelity results for all B-spline surrogates are listed in Table \ref{tab:ins_k2204_ppv_bsplines_surrogates_perf} .

\begin{table}

\centering \scriptsize
\begin{tabular}[t]{l|r|r|r|r|r}
\hline
  & $R^2$ & MSE & MAE & max AE & n leaves\\
\hline
B-spline baseline model & 0.9943260 & 0.9604583 & 0.7605289 & 4.249894 & 1\\
\hline
SLIM shallow & 0.9994172 & 0.0986492 & 0.2046541 & 1.880490 & 8\\
GUIDE shallow & 0.9993896 & 0.1033306 & 0.2132615 & 1.849715 & 8\\
MOB shallow & 0.9992104 & 0.1336634 & 0.2494695 & 2.063691 & 8\\
CTree shallow & 0.9990906 & 0.1539409 & 0.2713325 & 2.069590 & 8\\
\hline
SLIM deep & 0.9997505 & 0.0422310 & 0.1208647 & 1.421309 & 21\\
GUIDE deep & 0.9997299 & 0.0457276 & 0.1315567 & 1.307047 & 20\\
MOB deep & 0.9996846 & 0.0533855 & 0.1510094 & 1.342777 & 21\\
CTree deep & 0.9997083 & 0.0493729 & 0.1451053 & 1.385141 & 20\\
\hline
\end{tabular}
\label{tab:ins_k2204_ppv_bsplines_surrogates_perf}
\caption{Fidelity of K2204 PPV B-spline baseline model and  B-spline MBTs}
\end{table}





Table \ref{tab:ins_k2204_ppv_bsplines_surrogates_share} shows the proportions of observations that were split according to the different features. 


\begin{table}[!htb]
\centering \scriptsize
\begin{tabular}[t]{l|r|r|r}
\hline
  & age & duration & sex\\
\hline
SLIM shallow & 0.38 & 0.62 & 0.00\\
GUIDE shallow & 0.30 & 0.70 & 0.00\\
MOB shallow & 0.08 & 0.84 & 0.08\\
CTree shallow & 0.23 & 0.71 & 0.07\\
\hline
SLIM deep & 0.35 & 0.60 & 0.04\\
GUIDE deep & 0.20 & 0.78 & 0.02\\
MOB deep & 0.08 & 0.76 & 0.16\\
CTree deep & 0.20 & 0.67 & 0.13\\
\hline
\end{tabular}
\label{tab:ins_k2204_ppv_bsplines_surrogates_share}
\caption{Share of observations split by the different features K2204 PPV B-spline MBTs}
\end{table}



\begin{figure}[!htb]
    \centering   
    \includegraphics[width = 16cm]{Figures/insurance_use_case/k2204_PPV/slim_bsplines_small_tree.png}
    \caption{SLIM tree for K2204 PPV with B-spline models}
    \label{fig:ins_k2204_ppv_slim_bsplines_tree}
\end{figure}



\begin{figure}[!htb]
    \centering
    \includegraphics[width = 16cm]{Figures/insurance_use_case/k2204_PPV/effects_duration.png}
    \caption{Input-output relation of features in nodes split by duration for SLIM tree with B-splines and depth 3}
    \label{fig:ins_k2204_ppv_effects_duration}
\end{figure}




\begin{figure}[!htb]
    \centering    
    \includegraphics[width = 16cm]{Figures/insurance_use_case/k2204_PPV/effects_age_low_duration.png}
    \caption{Input-output relation of features in nodes with duration $\leq 25$ split by age for SLIM tree with B-splines and depth 3}
    \label{fig:ins_k2204_ppv_effects_age_low_duration}
\end{figure}

\begin{figure}[!htb]
    \centering    
    \includegraphics[width = 16cm]{Figures/insurance_use_case/k2204_PPV/effects_age_medium_duration.png}
    \caption{Input-output relation of features in nodes with $25 > $duration $<= 40$ split by age for SLIM tree with B-splines and depth 3}
    \label{fig:ins_k2204_ppv_effects_age_medium_duration}
\end{figure}


\begin{table}[!htb]

\centering \scriptsize
\begin{tabular}[t]{l|r|r|r|r}
\hline
  & $R^2$ & MSE & MAE & max AE \\
\hline
SLIM & 0.9997757 & 0.0383432 & 0.1140380 & 1.3335727\\
Blackbox model & 0.9998305 & 0.0289638 & 0.1060365 & 0.5345493\\
\hline
\end{tabular}
\label{tab:ins_k2204_ppv_standalone_slim}
\caption{Accuracy of standalone B-spline SLIM MBTs and of the black box model K2204 PPV}
\end{table}
